# Supplementary material for: Privileged observations enable rapid and reliable policy discovery directly in the physical world
Source: arXiv:2512.08463 source file (2026-09-11)
Supplement: Supplementary file 2 [file Supplementary_Figure_2.tex]

\includegraphics[width=\linewidth]{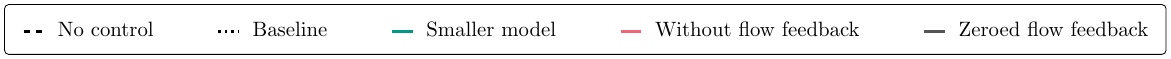}

    \begin{minipage}{.49\linewidth}
    \PFFPanelLetter{a}
    \includegraphics[width=\linewidth]{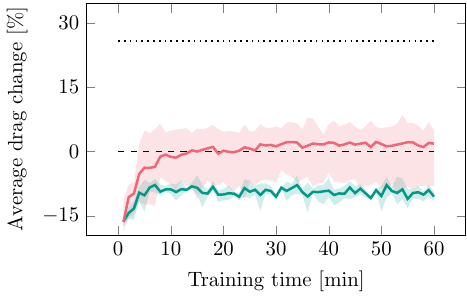}

    \end{minipage}
\hfill
    \begin{minipage}{.49\linewidth}
    \PFFPanelLetter{b}
    \includegraphics[width=\linewidth]{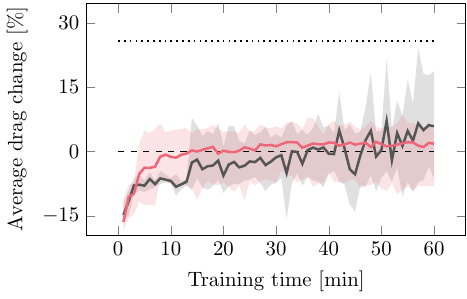}

    \end{minipage}
