# Supplementary material for: Privileged observations enable rapid and reliable policy discovery directly in the physical world
Source: arXiv:2512.08463 source file (2026-09-11)
Supplement: Supplementary file 3 [file Supplementary_Figure_3.tex]

\includegraphics[height=0.8cm]{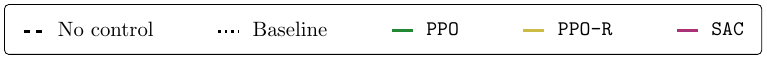}

    \begin{minipage}{.49\linewidth}
    \centering
        \PFFPanelLetter{a}
\includegraphics[width=\linewidth]{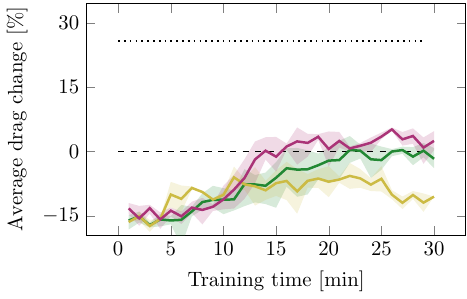}
    \end{minipage}
    \hfill
    \begin{minipage}{.49\linewidth}
    \centering
        \PFFPanelLetter{b}
\includegraphics[width=\linewidth]{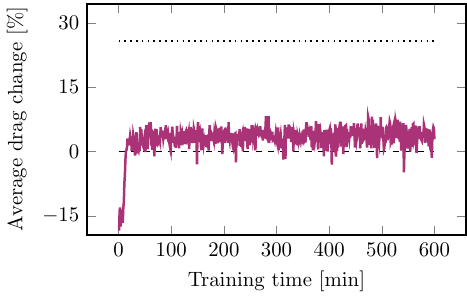}
    \end{minipage}
